# Supplementary material for: InstructABSA: Instruction Learning for Aspect Based Sentiment Analysis
Source: arXiv:2302.08624 source file (2023-11-13)
Supplement: Supplementary file 1 [file appendix_data_eff.tex]

\begin{table*}[]
\centering
\begin{tabular}{l|rrr|rrr|rrr}
\hline
\multicolumn{1}{c|}{Tasks}       & \multicolumn{3}{c|}{ATE}                                                                      & \multicolumn{3}{c|}{ATSC}                                                                     & \multicolumn{3}{c}{Joint}                                                                    \\ \hline
\multicolumn{1}{c|}{Size} & \multicolumn{1}{c|}{VanillaT5} & \multicolumn{1}{c|}{Tk-Instruct} & \multicolumn{1}{c|}{Diff} & \multicolumn{1}{c|}{VanillaT5} & \multicolumn{1}{c|}{Tk-Instruct} & \multicolumn{1}{c|}{Diff} & \multicolumn{1}{c|}{VanillaT5} & \multicolumn{1}{c|}{Tk-instruct} & \multicolumn{1}{c}{Diff} \\ \hline
10\%                             & \multicolumn{1}{r|}{57.06}     & \multicolumn{1}{r|}{71.81}       & 14.75                     & \multicolumn{1}{r|}{87.50}      & \multicolumn{1}{r|}{81.22}       & -6.28                     & \multicolumn{1}{r|}{50.31}     & \multicolumn{1}{r|}{57.50}        & 7.19                     \\
20\%                             & \multicolumn{1}{r|}{66.12}     & \multicolumn{1}{r|}{74.06}       & 7.94                      & \multicolumn{1}{r|}{85.76}     & \multicolumn{1}{r|}{85.12}       & -0.64                     & \multicolumn{1}{r|}{61.18}     & \multicolumn{1}{r|}{64.31}       & 3.13                     \\
50\%                             & \multicolumn{1}{r|}{77.50}      & \multicolumn{1}{r|}{82.37}       & 4.87                      & \multicolumn{1}{r|}{86.44}     & \multicolumn{1}{r|}{87.50}        & 1.06                      & \multicolumn{1}{r|}{68.40}      & \multicolumn{1}{r|}{69.87}       & 1.47                     \\
100\%                            & \multicolumn{1}{r|}{81.12}     & \multicolumn{1}{r|}{84.88}       & 3.76                      & \multicolumn{1}{r|}{87.33}     & \multicolumn{1}{r|}{89.64}       & 2.31                      & \multicolumn{1}{r|}{73.18}     & \multicolumn{1}{r|}{73.62}       & 0.44                     \\ \hline
\end{tabular}
\caption{Comparison of data efficiency achieved }
\end{table*}
